# Supplementary material for: Dealing with Controversy: An Emotion and Coping Strategy Corpus Based on Role Playing
Source: arXiv:2409.19025 source file (2024-09-26)
Supplement: Supplementary file 1 [file descriptions-pretest-round1.tex]

\begin{table*}
    \begin{tabularx}{\textwidth}{p{2cm}p{12.5cm}}
\toprule
\textbf{Strategy} & \textbf{Description}\\
\cmidrule(r){1-1}\cmidrule(r){2-2}
Attack & X does not shy away from unpleasant situations. When things are bad, X  invests significant effort in understanding why. Why did they go that way? This character is inclined to identify causes of discomfort, to confront them head-on, and attempt to rectify their consequences. That is when one can see X all tense and pumped up, committed to overcome an obstacle hindering a better life.

Injustice hurts X profoundly. This character affirms what bothers it by facing the source of stress directly and aggressively. Always ready to right the wrong, X takes action to change the situation, and can come across as attacking. But this severity does not only apply to others: if X is responsible for their failures or something wrong, X reproaches itself.\\
\cmidrule(r){1-1}\cmidrule(r){2-2}
Contact & This character possesses a constructive, problem-solving mindset. X expresses ideas and desires with confidence, striving to achieve practical objectives. X understands the importance of self-worth.

For X, communication serves to unite people. It is an opportunity to exchange opinions openly and respectfully, acknowledging the diversity of perspectives among individuals. X can effectively engage in discussions also with people holding contrasting opinions. 

X maintains this attitude even in the context of unpleasant situations: X engages with the source of stress in a proactive manner, coming across as a very approachable person.\\
\cmidrule(r){1-1}\cmidrule(r){2-2}
Distance & This character is avoidant. Unpleasant events make X feel powerless, as if the potential repercussions were entirely uncontrollable. X thinks there's not much one can do to change the external world. One can act on oneself, though.

For X, tense, confrontational exchanges with other people are not a source of excitement. Accompanied by a sense of anxiety, this person has developed a strong defence strategy to deflect focus from stressful things, events, people or thoughts: keeping oneself away from all wrongdoings (both personal and of others). Conflicts and uncomfortable situations should be avoided at all costs, with the effort to minimise their negative influence in one's life. \\
\cmidrule(r){1-1}\cmidrule(r){2-2}
Reject & ``No time for fools, it's best to keep one's distance from other people''. This is a typical way of thinking of X, a person who does not easily approach or trust others. X believes that nobody can get an important job done: it's best to work and be alone, even if that creates some distance with the rest of the world.

This person is prone to being displeased, ready to wrinkle in aversion. X would really prefer not to be involved in any difficult situation. In fact, X withdraws from any circumstance mismatching personal goals or preferences, and tries to minimise the engagement with the cause of such distress. This character tends to deny the influence of unpleasant, negative things. If there were one motto in life, X's would be: bring yourself in a state of peace.\\
\bottomrule
\end{tabularx}
\caption{Descriptions used in the pre-test, for Round 1.}
\label{pre-study-descriptions-1}
\end{table*}
