# Supplementary material for: Dealing with Controversy: An Emotion and Coping Strategy Corpus Based on Role Playing
Source: arXiv:2409.19025 source file (2024-09-26)
Supplement: Supplementary file 2 [file descriptions-pretest-round2.tex]

\begin{table*}
    \begin{tabularx}{\textwidth}{p{2cm}p{12.5cm}}
\toprule
\textbf{Strategy} & \textbf{Description}\\
\cmidrule(r){1-1}\cmidrule(r){2-2}
Attack & When unpleasant situations arise, X responds with a hardened resolve. This character does not seek consolation or advice from others, but instead confronts problems head-on, often with an aggressive and intense energy. X's approach to overcoming obstacles is a solo fight to right the wrong.

Injustice hurts X profoundly; unfairness is a trigger, igniting a spark that pushes this character to face the source of stress directly and fiercely. Why did things go that way? X is driven to identify the causes of discomfort, to confront them head-on, in the attempt to rectify their consequences.

X, who does not shy away from conflicts, takes action to change negative situations in a proactive manner, and can come across as combative. That is when one can see X all tense and pumped up, committed to overcome an obstacle. This resolution isn't only aimed outwards; if X perceives personal failure or wrongdoing, it has a tendency to self-criticize and demand more. \\
\cmidrule(r){1-1}\cmidrule(r){2-2}
Reject & This person, who does not easily trust others, is prone to being displeased, always ready to wrinkle in aversion. So here's how X approaches life: the world is simpler when one refuses to engage in negativity. A striking characteristic of X is this ability to deflect interactions that could result in conflict. One could almost say that unpleasant events do not concern X's existence, because X has mastered the skill of rebuking circumstances that mismatch personal goals or preferences.

When faced with a source of potential distress, X effectively minimizes its importance or impact. This is not due to a lack of courage, but to a fundamental belief that it's better to completely repudiate all difficulties. For this character, personal tranquility rules above all else, and uncomfortable situations must be dismissed at all costs. \\

\bottomrule
\end{tabularx}
\caption{Descriptions used in the pre-test, for Round 2.}
\label{pre-study-descriptions-2}
\end{table*}
