# Supplementary material for: Dealing with Controversy: An Emotion and Coping Strategy Corpus Based on Role Playing
Source: arXiv:2409.19025 source file (2024-09-26)
Supplement: Supplementary file 3 [file descriptions-pretest-round3.tex]

\begin{table*}
    \begin{tabularx}{\textwidth}{p{2cm}p{12.5cm}}
\toprule
\textbf{Strategy} & \textbf{Description}\\
\cmidrule(r){1-1}\cmidrule(r){2-2}
Attack & When unpleasant situations arise, X responds with a hardened resolve. This character confronts problems head-on, often with an aggressive and intense energy. X's approach to overcoming obstacles is a solo fight to right the wrong.

Unfairness is a trigger for X, igniting a spark that pushes this character to fight the source of stress fiercely. Why did things go that way? X does not shy away from conflicts, and tries to identify the causes of discomfort in the attempt to rectify their consequences.

X takes action to change negative situations personally. For this reason, X can come across as combative. One can often see X tense and pumped up, committed to overcome an obstacle. This resolution isn't only aimed outwards; if X perceives personal failure or wrongdoing, it has a tendency to self-criticize and demand more. \\
\cmidrule(r){1-1}\cmidrule(r){2-2}
Contact & This character possesses a constructive, problem-solving mindset. X expresses ideas and desires with confidence, striving to achieve practical objectives. X understands the importance of self-worth.

For X, communication serves to unite people. It is an opportunity to exchange opinions openly and respectfully, acknowledging the diversity of perspectives among individuals. X can effectively engage in discussions also with people holding contrasting opinions. 

X maintains this attitude even in the context of unpleasant situations: X engages with the source of stress in a proactive manner, coming across as a very approachable person.\\
\cmidrule(r){1-1}\cmidrule(r){2-2}
Distance & This character is avoidant. Unpleasant events make X feel powerless, as if the potential repercussions were entirely uncontrollable. X thinks there's not much one can do to change the external world. One can act on oneself, though: rather than engaging in conflict or confrontations, X seeks emotional and mental space, finding solace in self-reflection.

For X, tense, confrontational exchanges with other people are not a source of excitement. Accompanied by a sense of anxiety, this person has developed a strong defense strategy to deflect focus from stressful things, events, people or thoughts: keeping oneself away from all wrongdoings (both personal and of others). Conflicts and uncomfortable situations should be avoided at all costs, with the effort to minimize their negative influence in one's life. \\
\cmidrule(r){1-1}\cmidrule(r){2-2}
Reject & This person easily disagrees with others, and has a quite judgmental attitude towards their behaviors and beliefs. For this reason X is often displeased, ready to wrinkle in aversion when people don't align with X's expectations.

For this character, uncomfortable situations must be dismissed at all costs. So here's X's approach to life: just let people with ideas that you dislike not interfere with your personal well-being -- not by aggressively facing them, but confidently let them know your position.

X tends to refuse negativity: all circumstances that mismatch personal goals or preferences can be turned down, not due to a lack of courage, but to a fundamental belief that it's better to solve difficulties by directly getting rid of them.\\
\bottomrule
\end{tabularx}
\caption{Descriptions used in the pre-test, for Round 3.}
\label{tab:pre-study-descriptions-3}
\end{table*}
